# Supplementary material for: Algorithms that "Don't See Color": Comparing Biases in Lookalike and Special Ad Audiences
Source: arXiv:1912.07579 source file (2022-05-31)
Supplement: Supplementary file 1 [file appendix.tex]

\section*{Appendix}

\setcounter{figure}{0}
